# Supplementary material for: Finite-Entanglement Scaling of 2D Metals
Source: arXiv:2305.02091 source file (2024-01-09)

$$|\psi_{\text{in}}\rangle$$
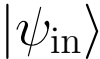

The diagram illustrates a quantum circuit. At the top, a horizontal line represents the input state  $|\psi_{\text{in}}\rangle$ . From this line, two vertical arrows point downwards to two separate square blocks, each labeled  $T_\epsilon$ . These blocks are arranged side-by-side. From the bottom of each  $T_\epsilon$  block, another vertical arrow points downwards, representing the output of each path.

$$T_\epsilon$$

$$T_\epsilon$$

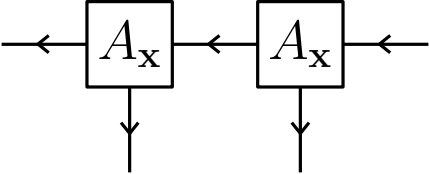

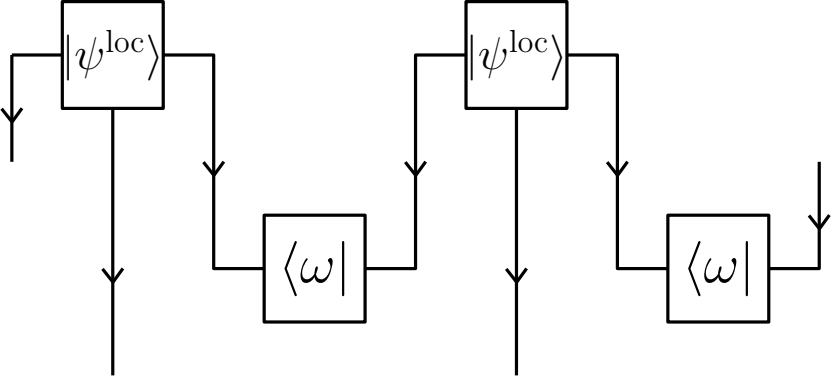

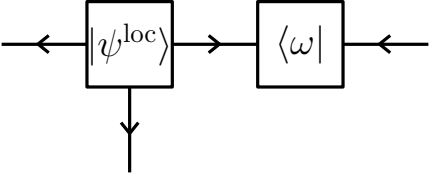

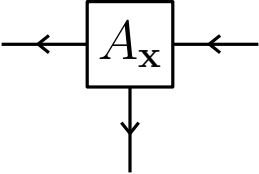

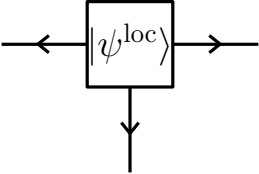

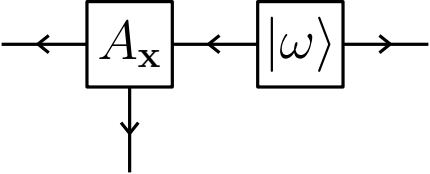

$\Psi$

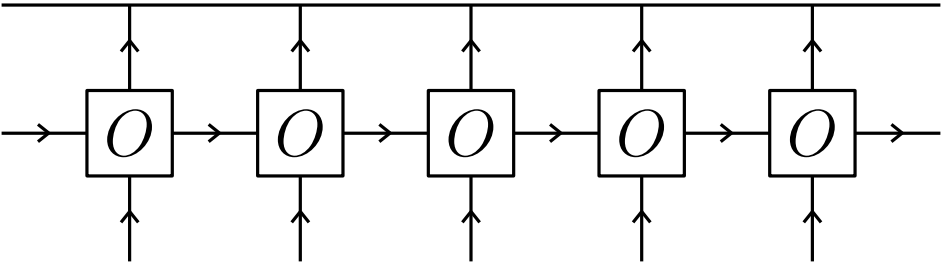



$\Psi$

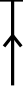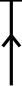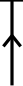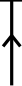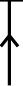

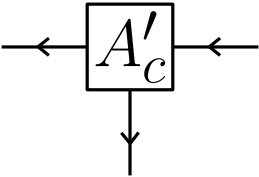

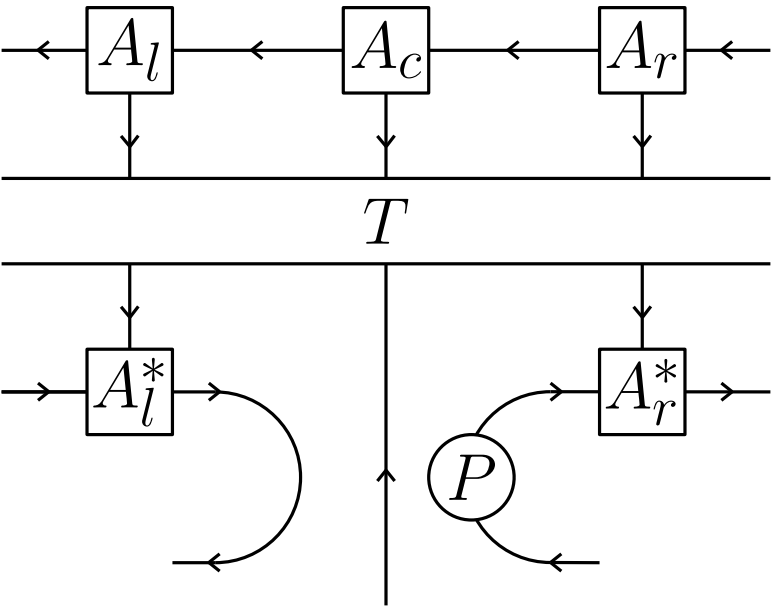

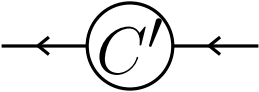

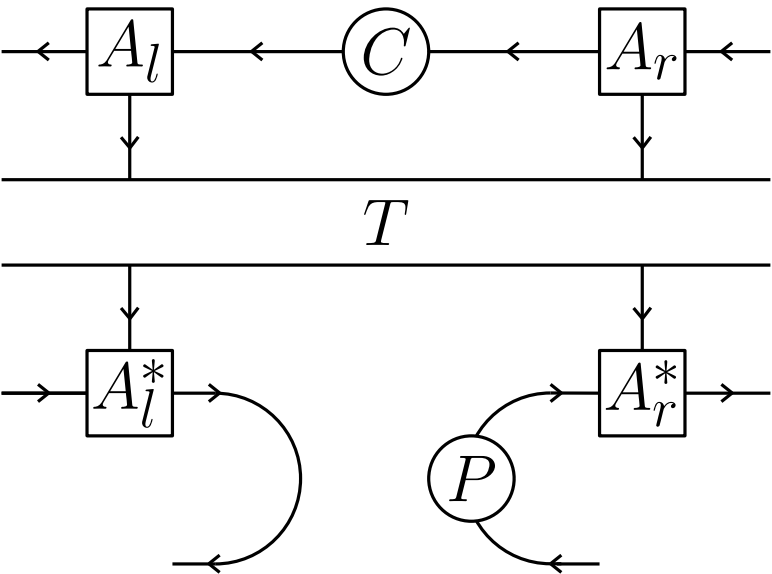

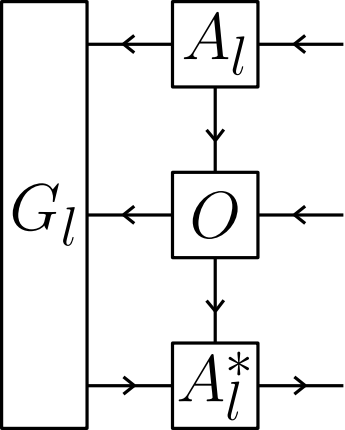

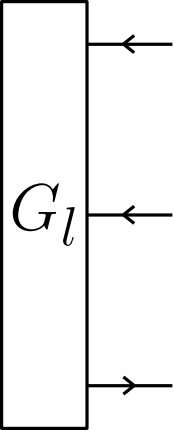

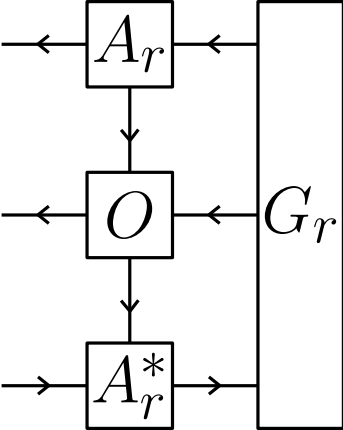



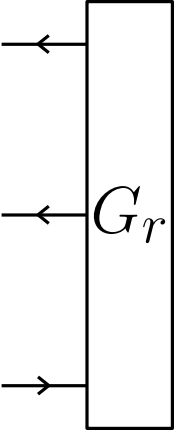

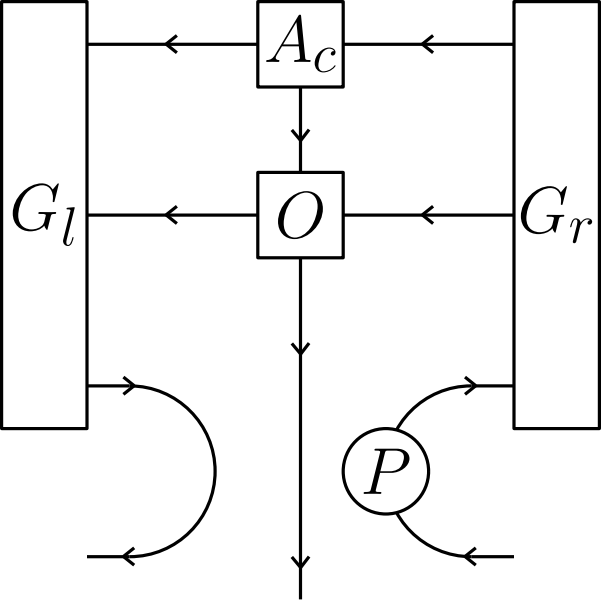

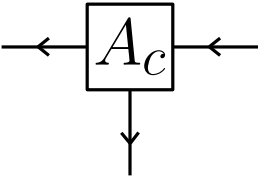

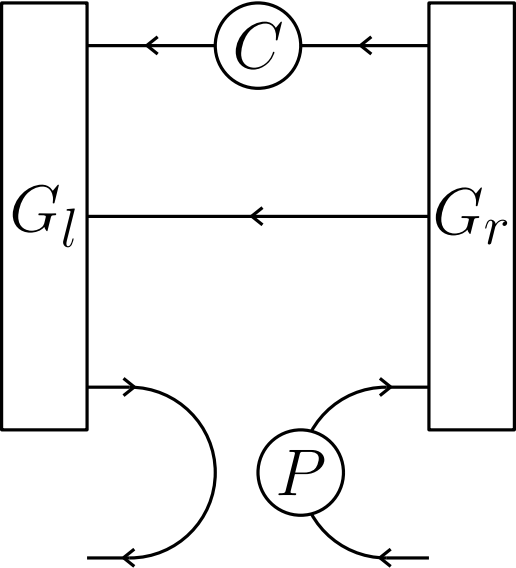

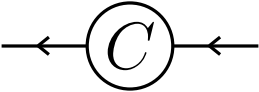

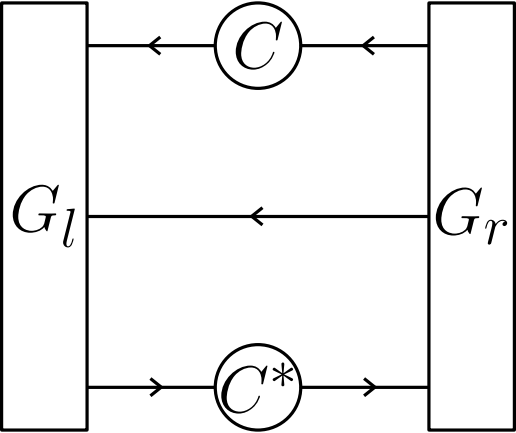

$\beta$

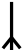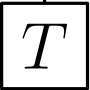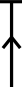

$\alpha$

$\alpha$

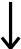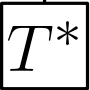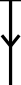

$\beta$



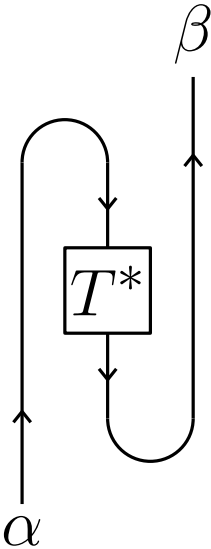

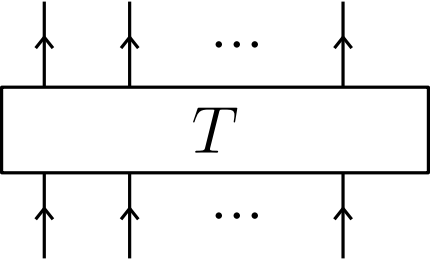

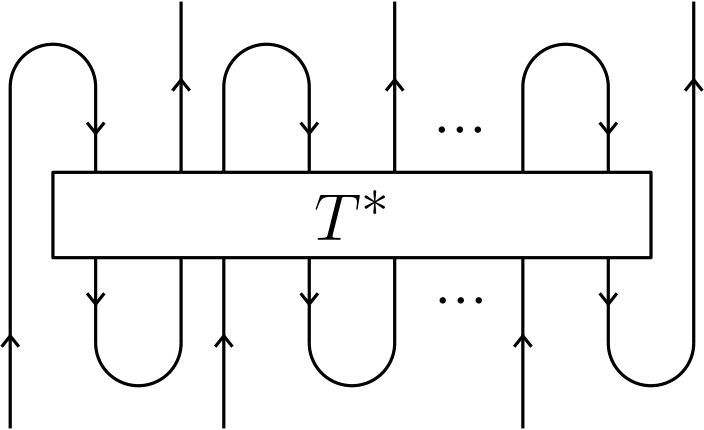

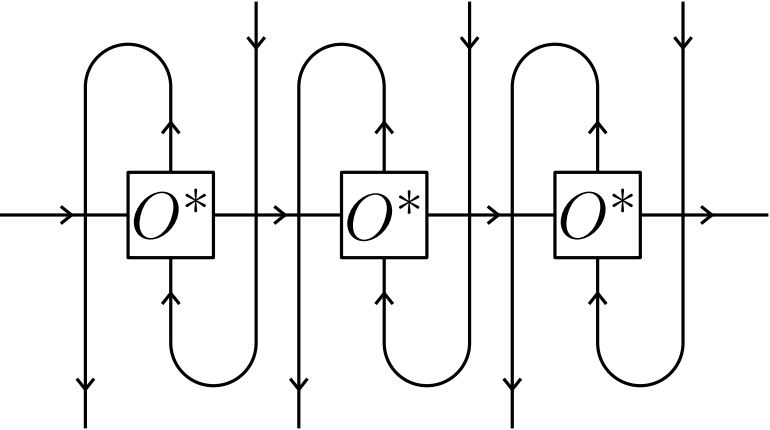

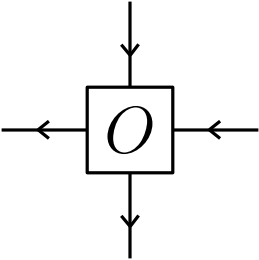

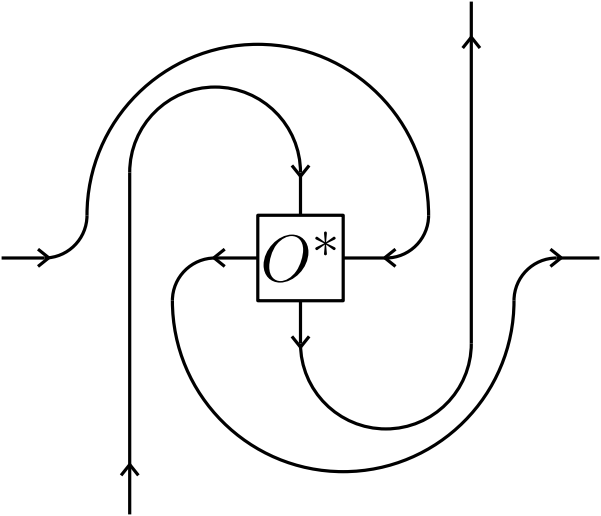

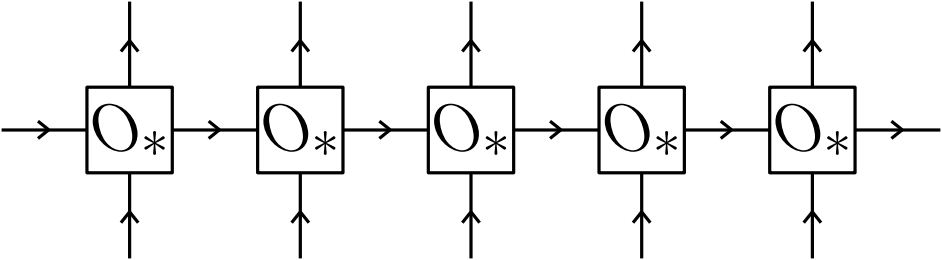

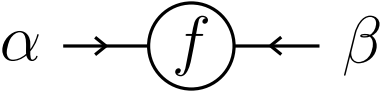



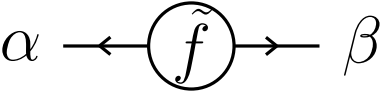

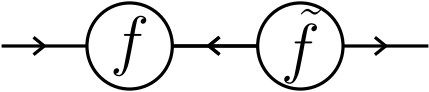

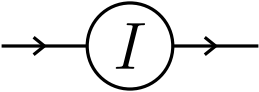

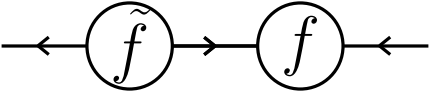

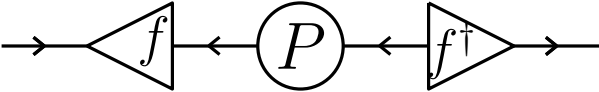

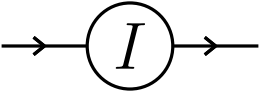

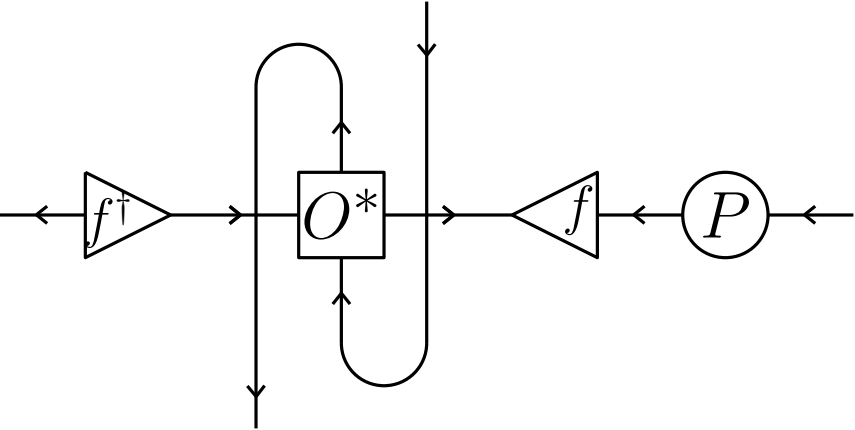

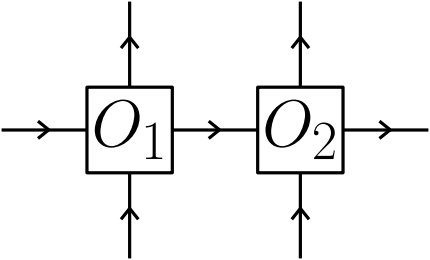



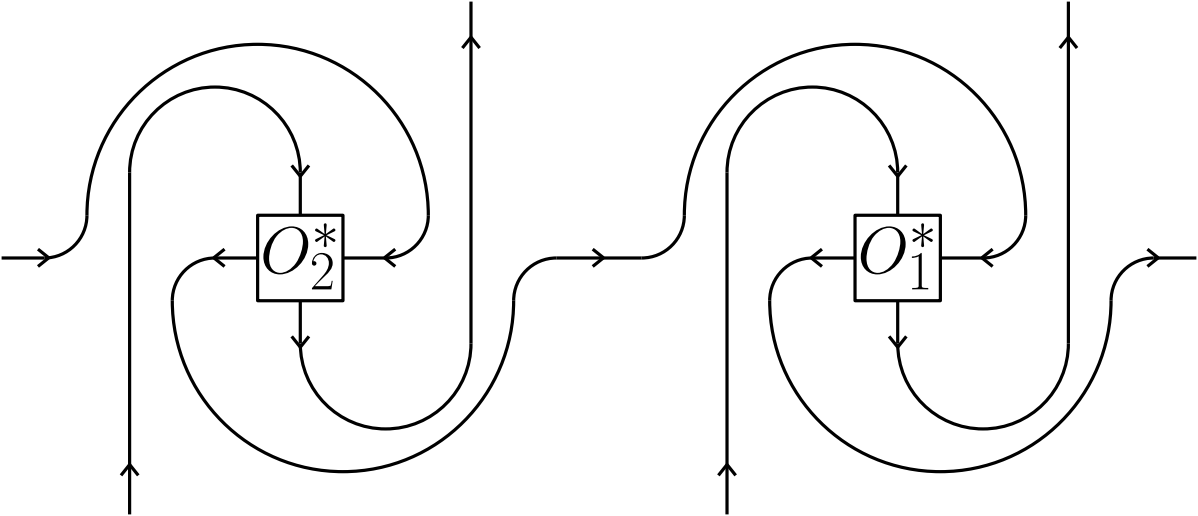

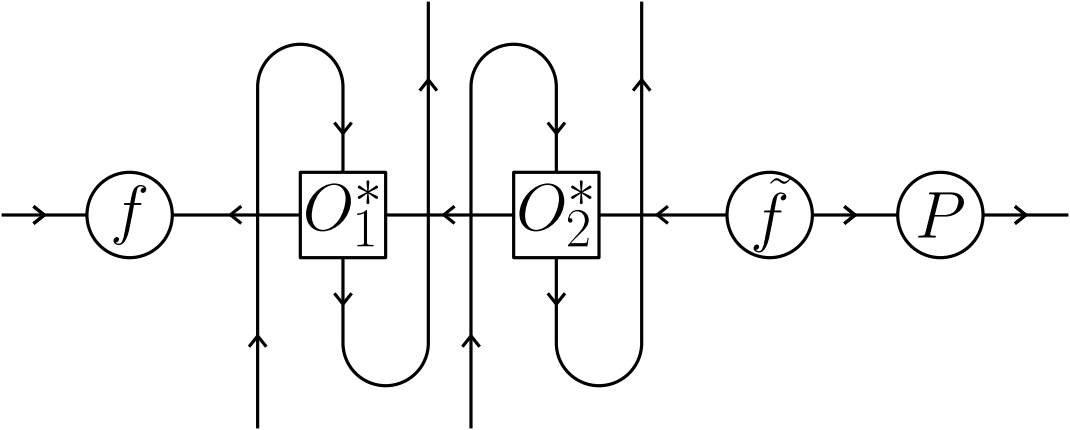

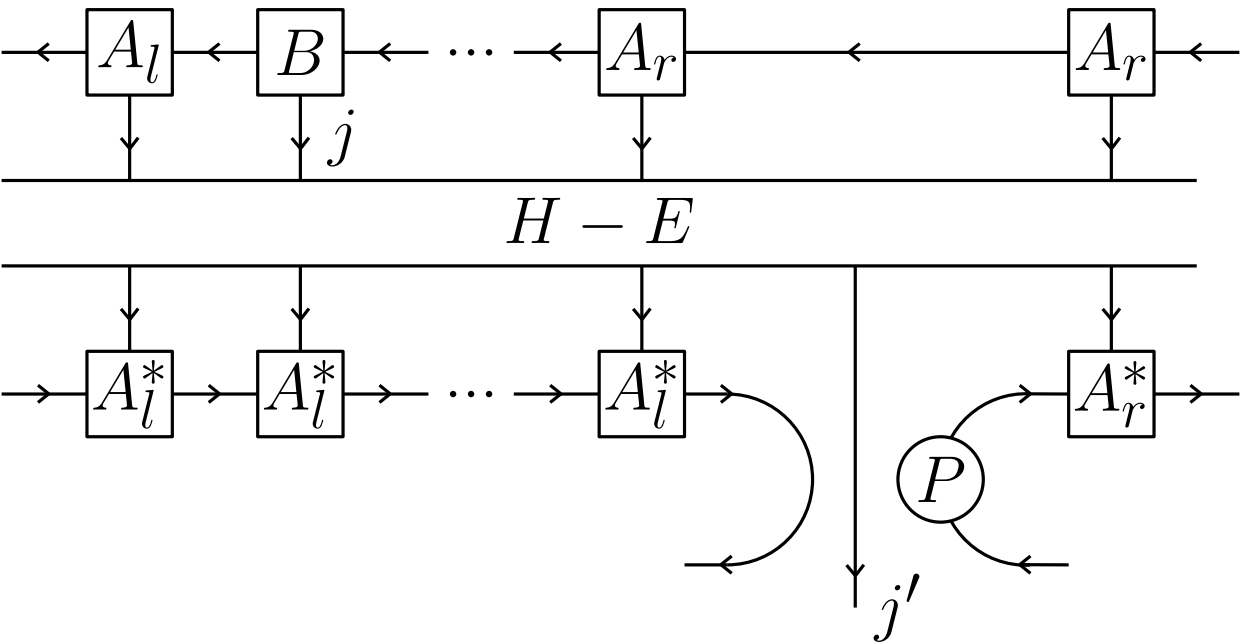

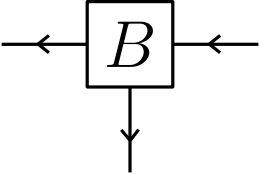

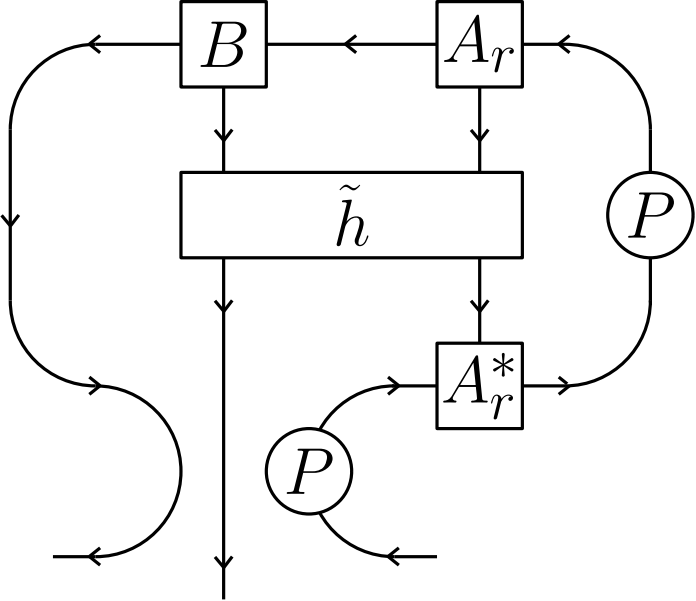

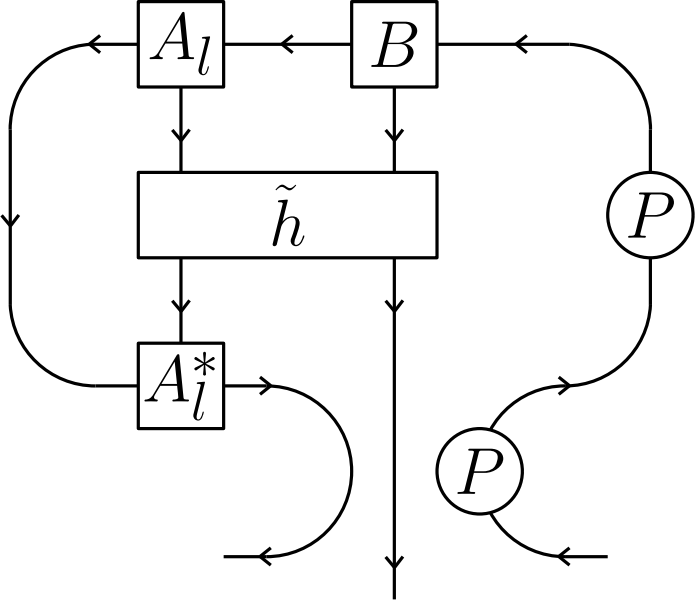

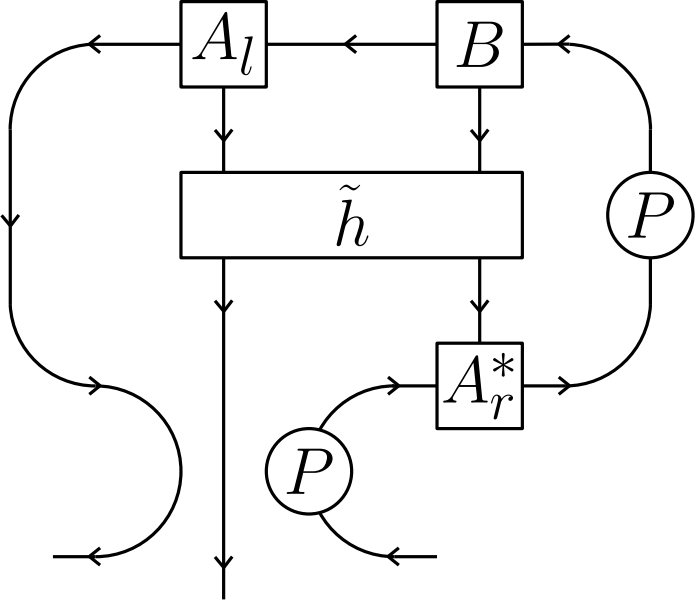

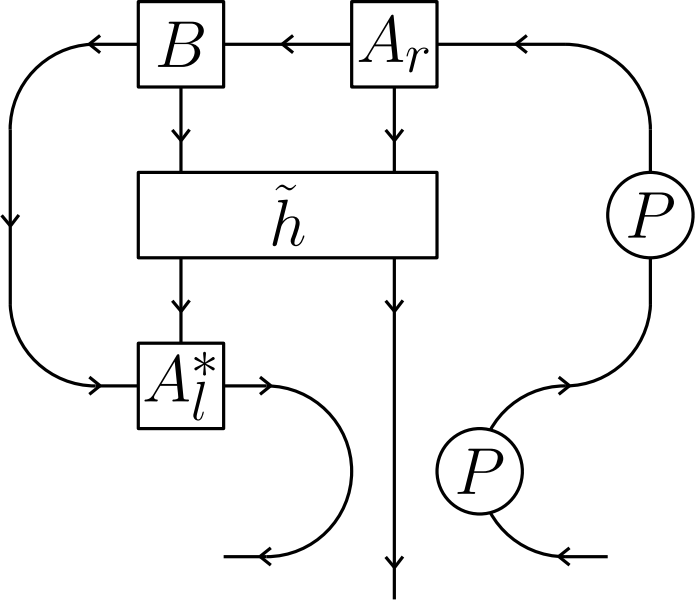



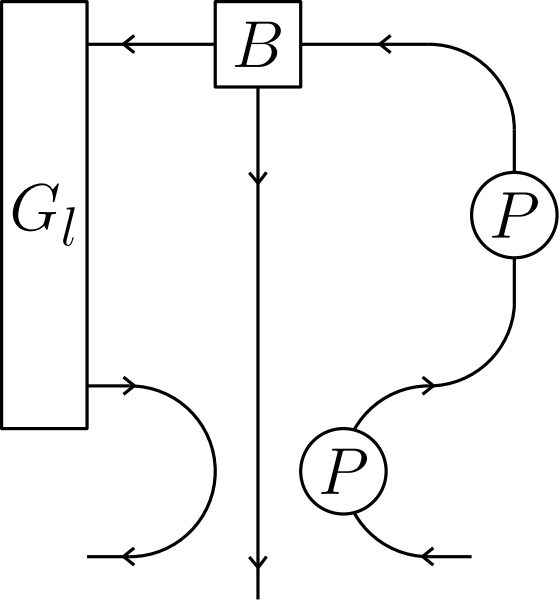

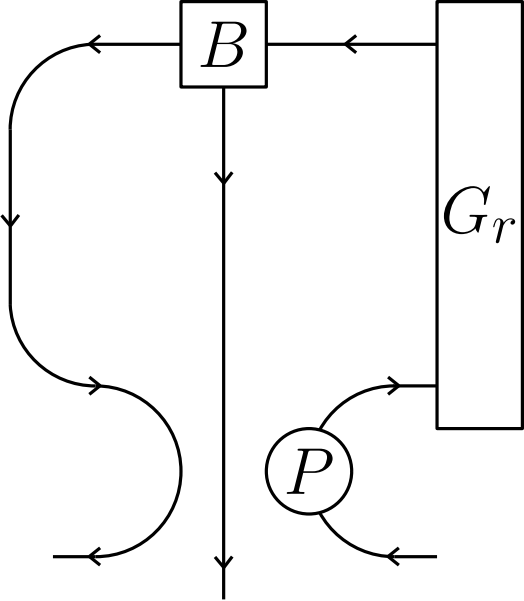

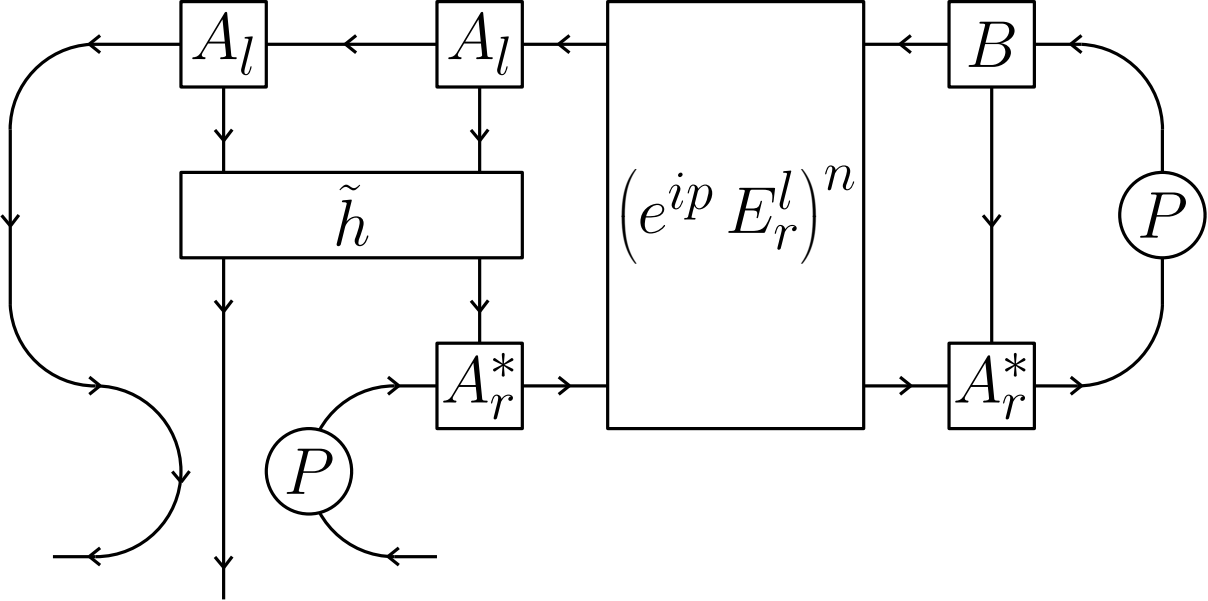

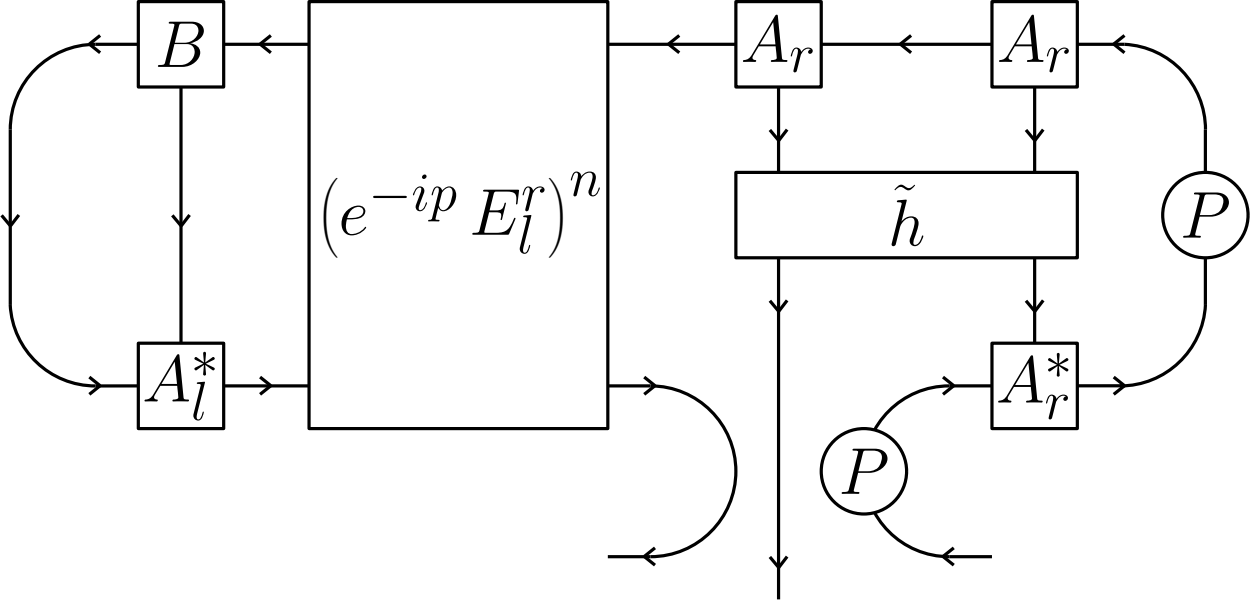

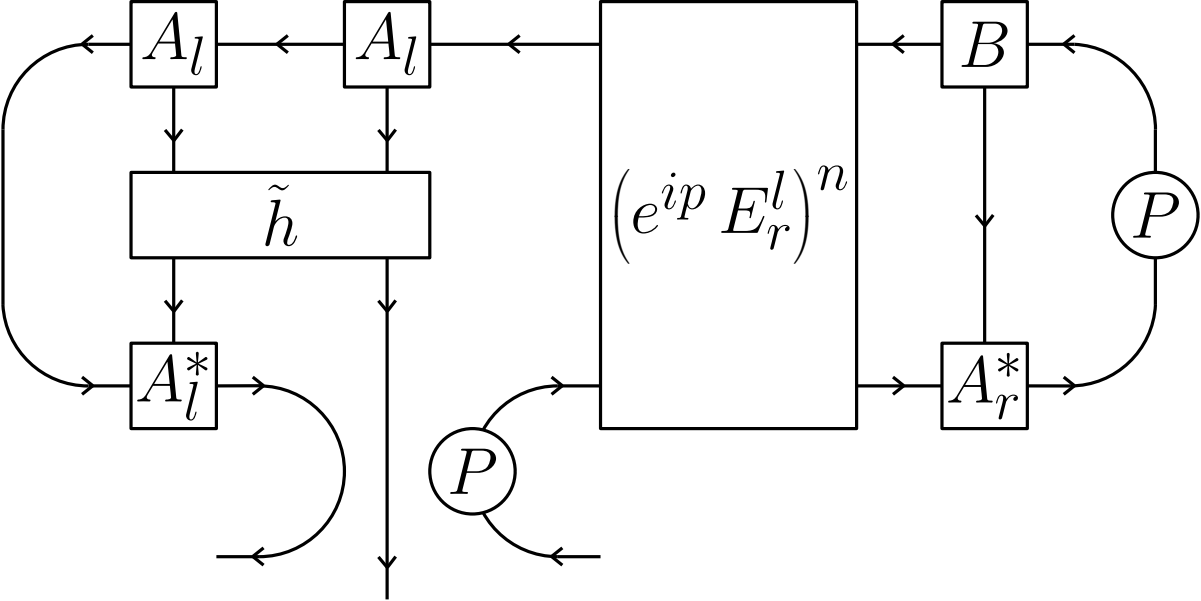

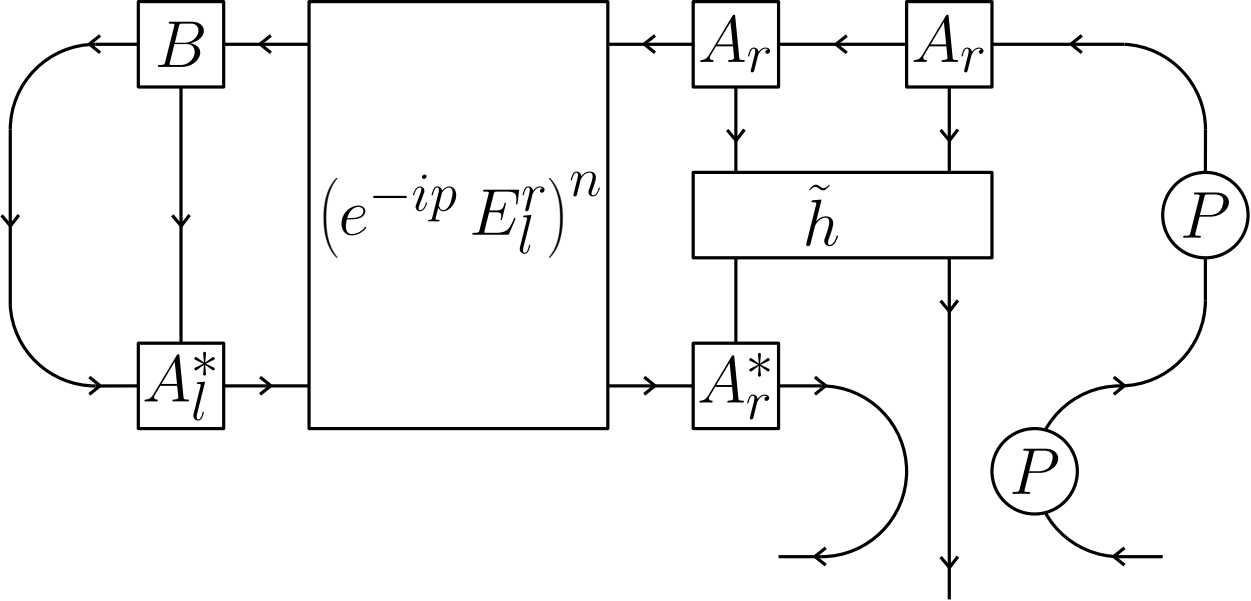

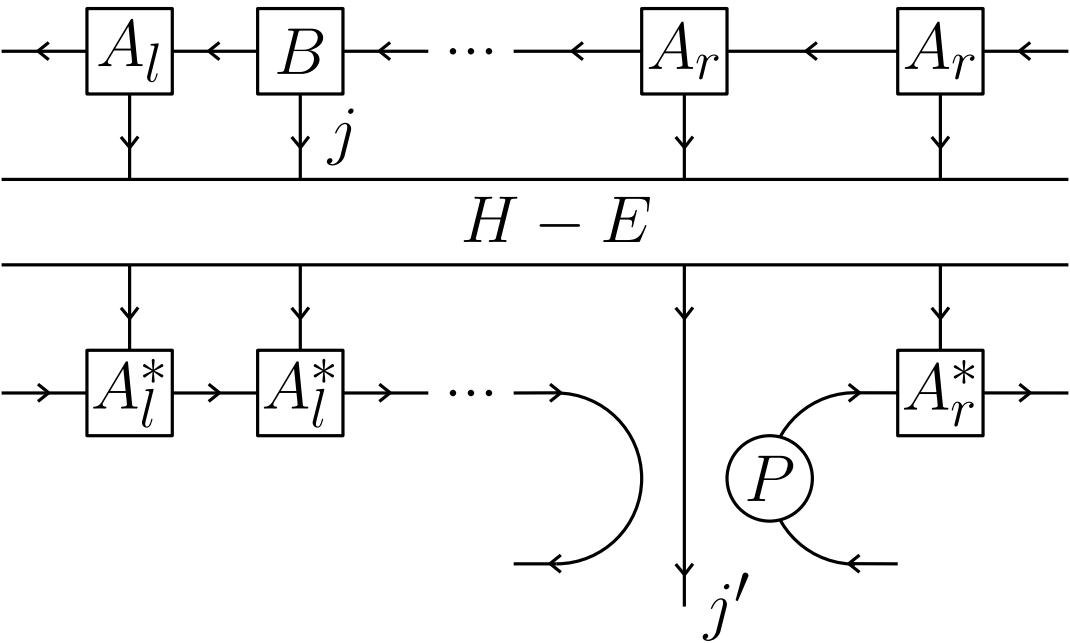

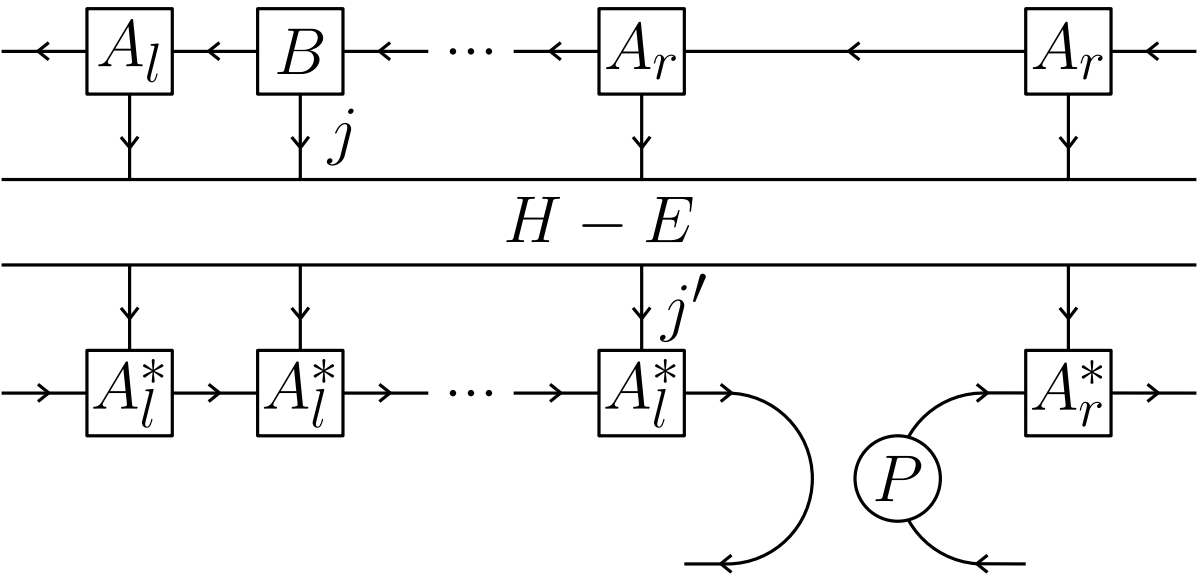



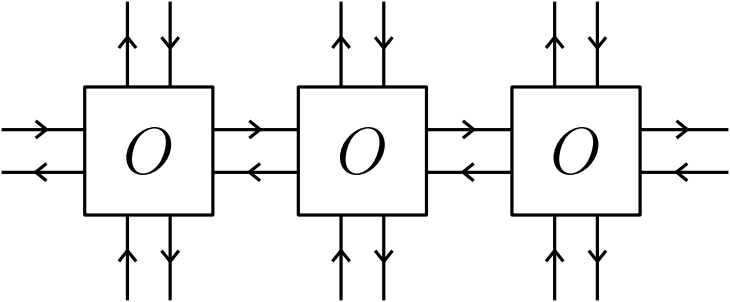

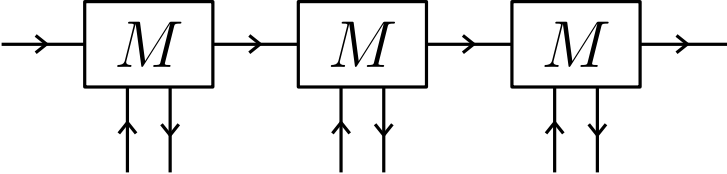

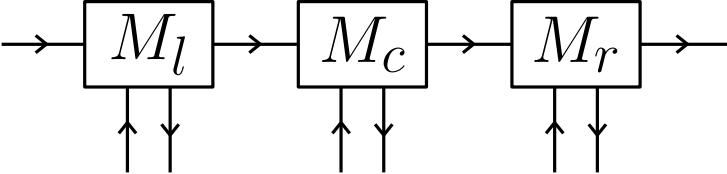

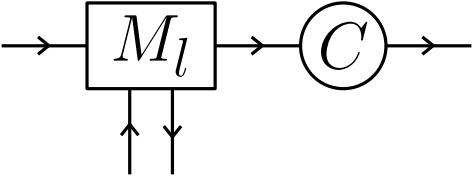

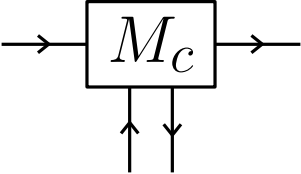

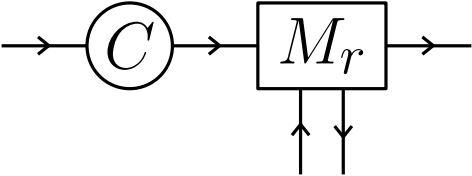

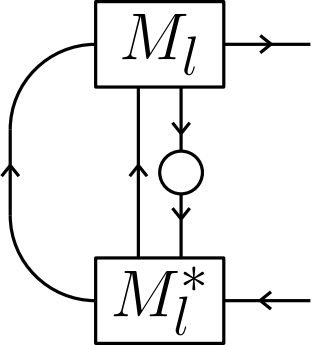

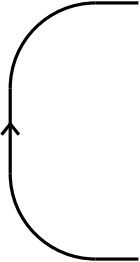



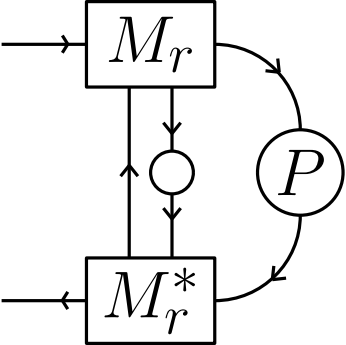

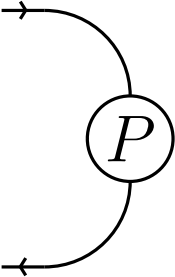

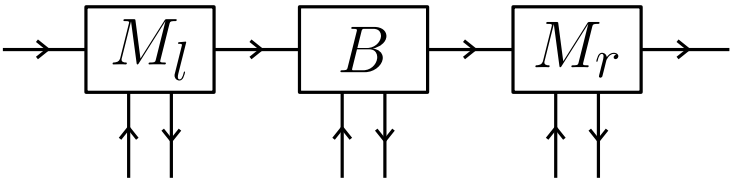

$j$

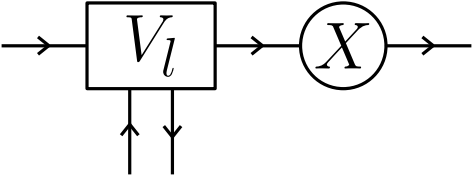

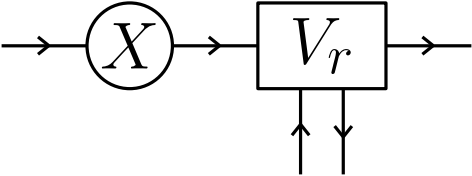

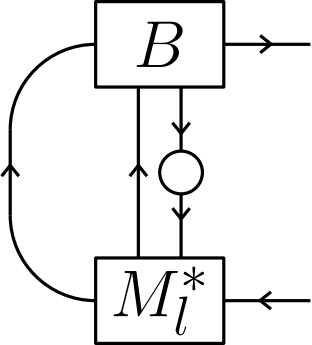

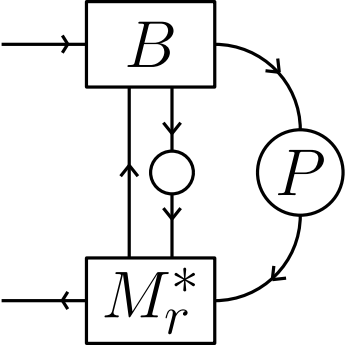

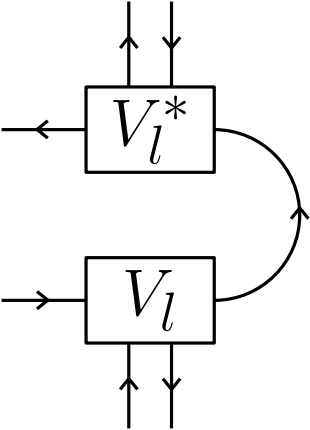



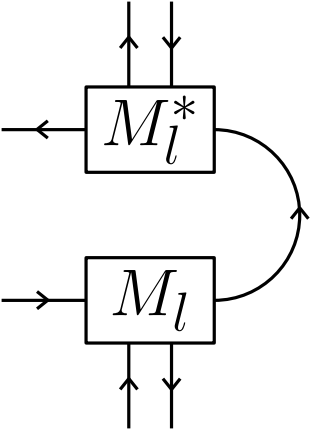

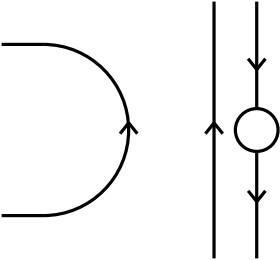

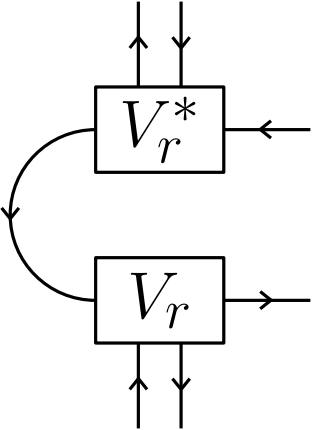

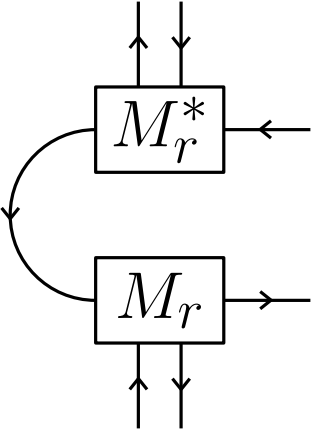

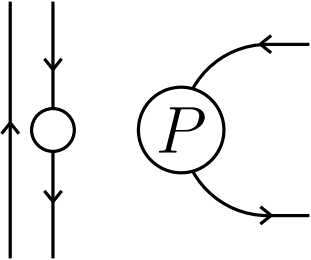

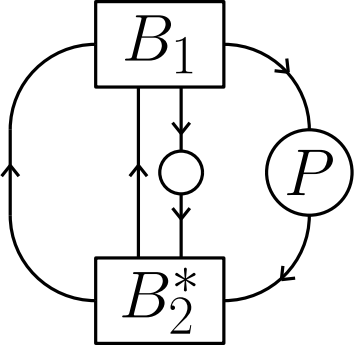

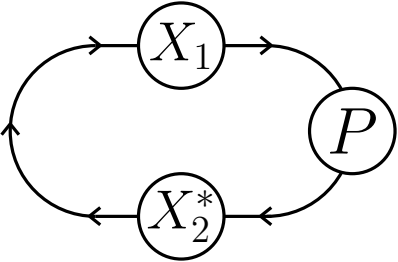

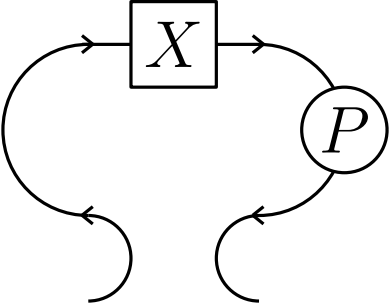



$\chi$

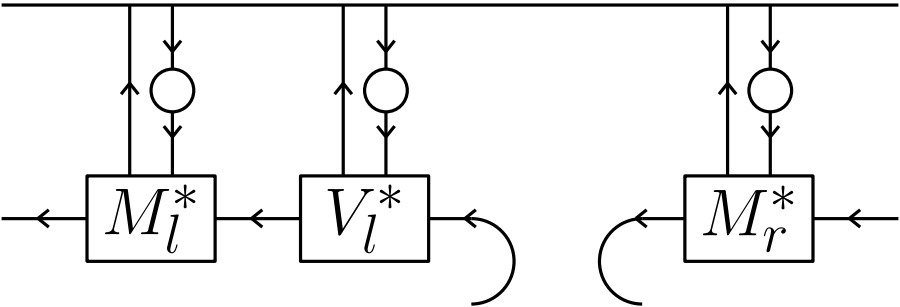

$M_r^*$

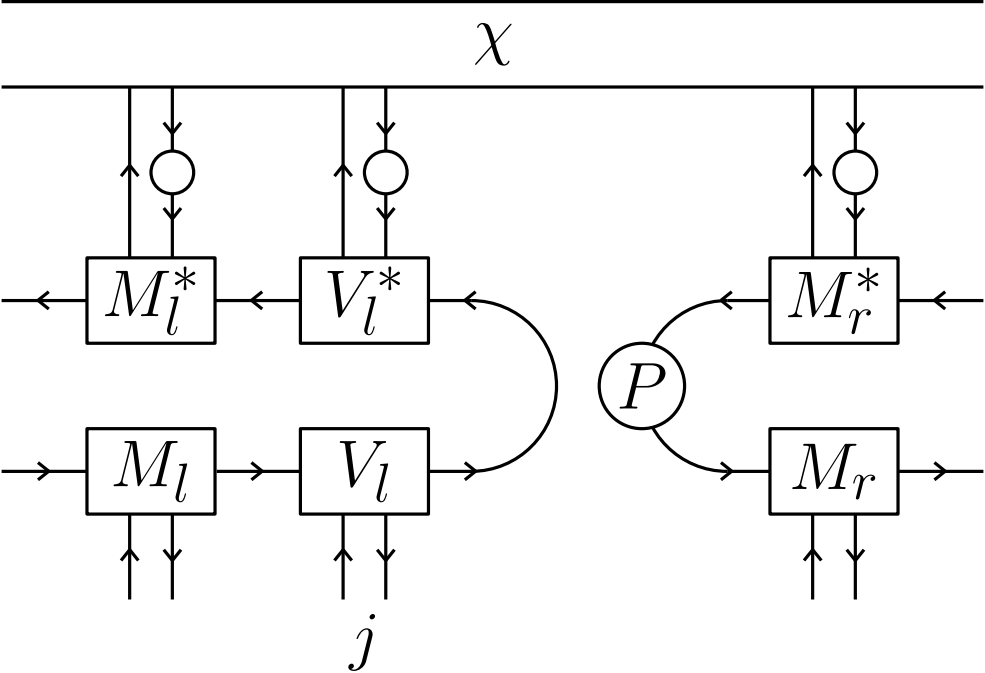

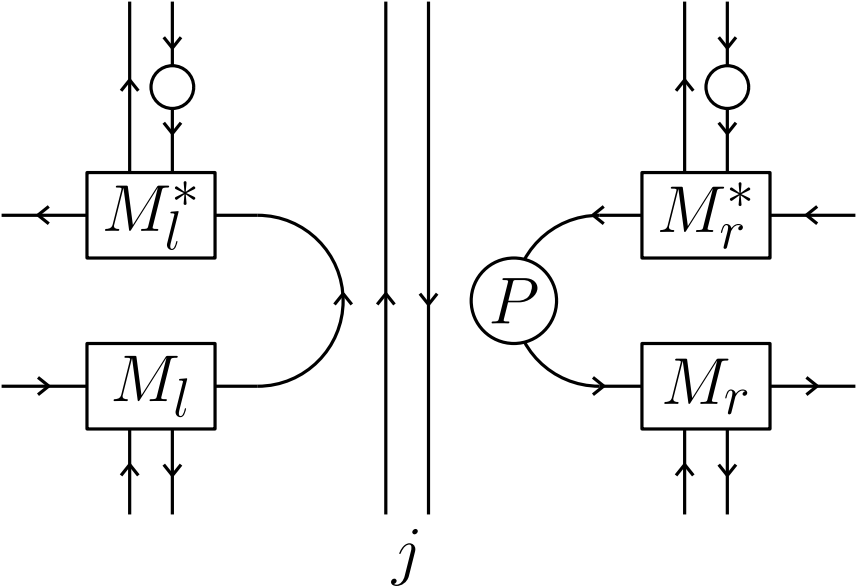

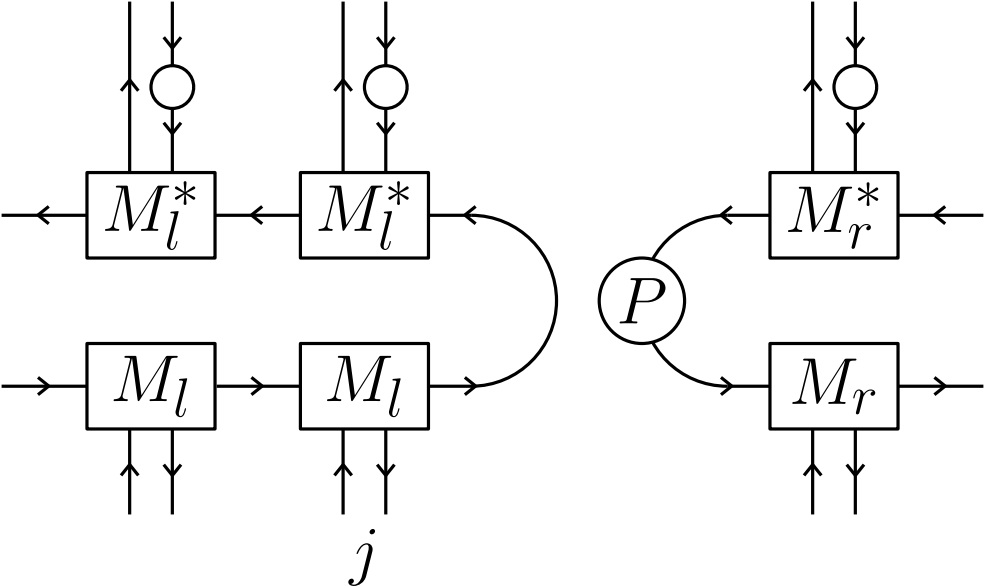

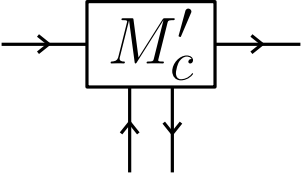

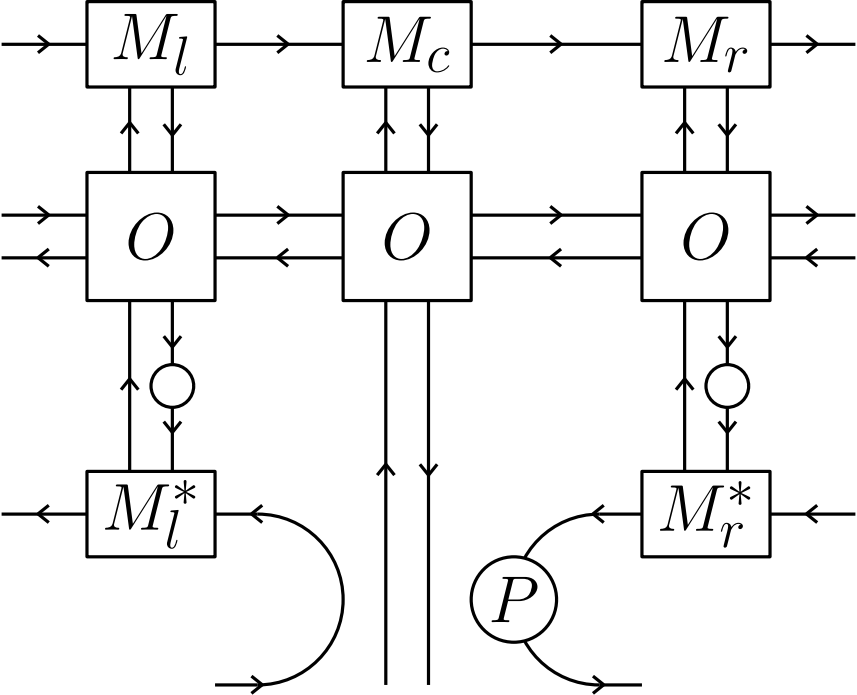

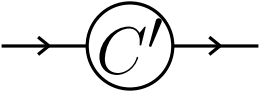

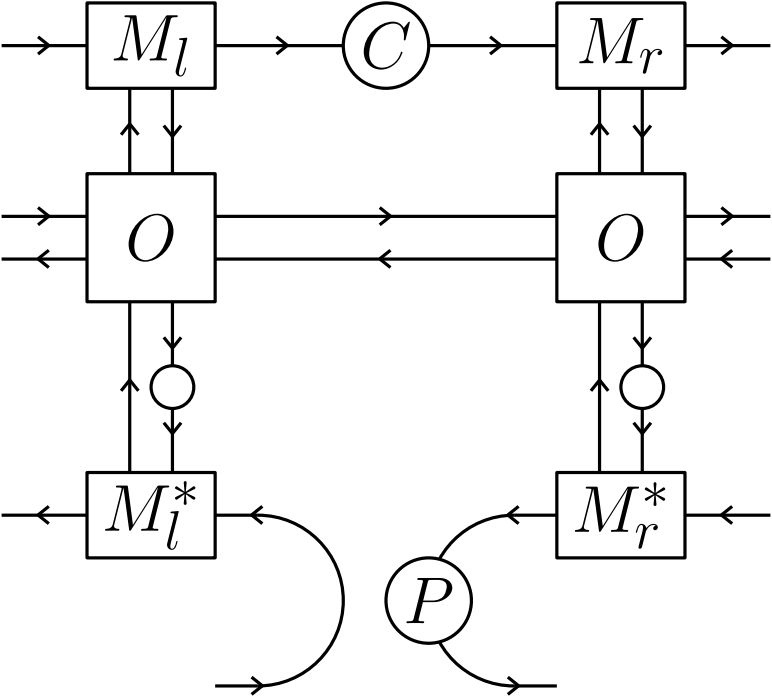



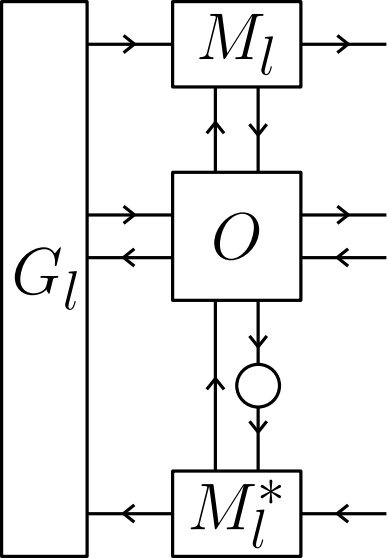

$G_l$

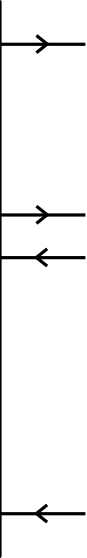

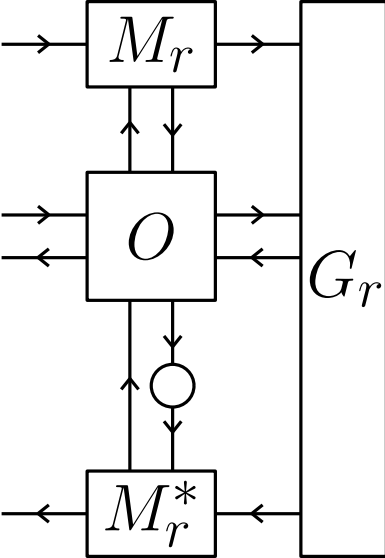

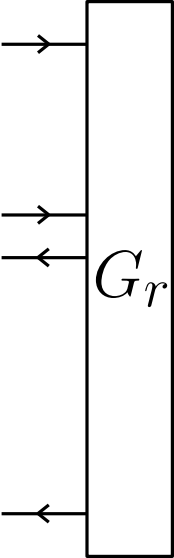

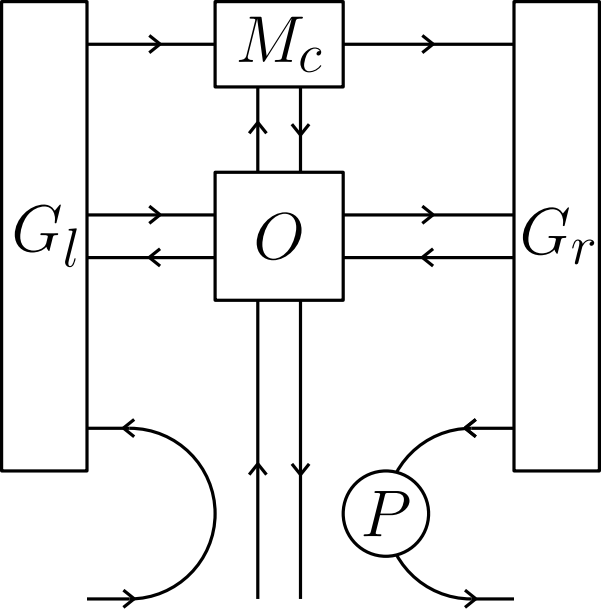

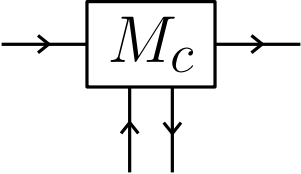

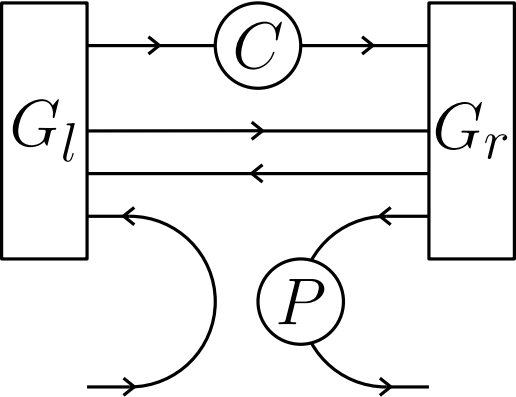

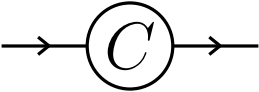



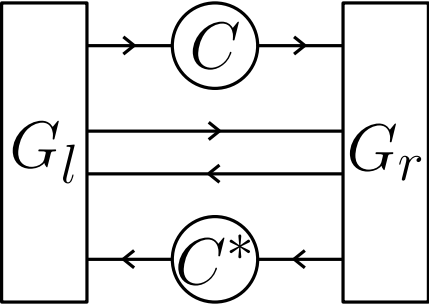

Supplement: Supplementary file 1 [file appendix.pdf]
